# Supplementary material for: Controllable Shape Modeling with Neural Generalized Cylinder
Source: arXiv:2410.03675 source file (2024-09-18)
Supplement: Supplementary file 1 [file supp_body.tex]

In this supplementary material, we first show details in the \textit{Method} section of main paper in Sec.~\ref{supp_method}. Then introduce the details in the \textit{Experiments} section of main paper in Sec.~\ref{supp_exp}. Finally, we discuss the implementation of shape generation with our \ReprName~ in Sec.~\ref{supp_generation}.

\section{Technical Details}
\label{supp_method}
In the section, we will introduce some technical details, including implementation of the central curve in \ReprName, which is related to discretization of curve and interpolation of radii and local frames. Then we discuss the detailed configuration in preprocessing, network structure and mesh extraction.

\subsection{Relative Coordinate System}
% How to implement the cylinder; nearest points edge case. 
\parahead{Interpolation} 
For choice of parameter $t$ for the piece-wise linear (PWL) curve, it is defined as the relative length of the path for a point. Specifically, assume $\Point$ is on the PWL curve, endpoints are $\Point_0$ for $t=0$ and $\Point_1$ for $t=1$. Then the parameter $t$ for $\Point$ is formulated as $\frac{\overline{\Point_0 \Point}}{\overline{\Point_0 \Point_1}}$, where $\overline{\Point_0 \Point}$ is length of the path from $\Point_0$ to $\Point$ and $\overline{\Point_0 \Point_1}$ is the total length of the curve.

Recall the implementation  of generalized cylinder (GC), we set $\mathbf{y}$ and $\mathbf{z}$ at key frames (e.g. $t \in \{ 0.0, 0.5, 1.0 \}$) and obtain rest $\mathbf{y}(t)$ and $\mathbf{z}(t)$ for other $t \in [0,1]$ by interpolation. For convenience, denote the $y$ and $z$ direction radius of $\textit{Profile}(t_i)$ as $r_y(t_i)$ and $r_z(t_i)$, where $t_i$ is one of the key frame. Denote as well the unitary local frame at $t_i$ is $\mathcal{F}(t_i)$. Let $\{ t_i \}_{i=1}^n$ be $n$ key frames of [0,1] in increasing order, and $t_1=0, t_n=1$. For any $t \in [0,1]$, we can compute its radius and frame as:
\begin{align*}
    r_y(t) &= \textit{Lerp} (t, \{ t_i \}_{i=1}^n, \{ r_y(t_i) \}_{i=1}^n), \\
    r_z(t) &= \textit{Lerp} (t, \{ t_i \}_{i=1}^n, \{ r_z(t_i) \}_{i=1}^n), \\
    \mathcal{F}(t) &= \textit{Slerp} (t, \{ t_i \}_{i=1}^n, \{ \mathcal{F}(t_i) \}_{i=1}^n).
\end{align*}
Here $\textit{Lerp}$ is linear interpolation, and $\textit{Slerp}$ is spherical linear interpolation. Basically, if $t \in (t_i, t_{i+1}]$, then $r_y(t) = \frac{t - t_i}{t_{i+1} - t_i} r_y(t_{i+1}) + \frac{t_{i+1} - t}{t_{i+1} - t_i} r_y(t_i)$, similarly for $r_z(t)$. For $\textit{Slerp}$, it interpolates the two rotation matrices $\mathcal{F}(t_i), \mathcal{F}(t_{i+1})$. We use the implementation of \textit{Scipy} for \textit{Slerp}.

\parahead{Closest point.}
For any point $\AnotherPoint$ inside the GC, there can be multiple closest points on the curve, since the optimization problem $t = \arg \min_t || \AnotherPoint - \Curve(t) ||_2$ is generally non-convex. To handle this case, we assume $\AnotherPoint$ has two closest points $\Point_1=\Curve(t_1), \Point_2=\Curve(t_2)$ on the curve, and their relative coordinates are $(t_1, a_1, b_1), (t_2, a_2, b_2)$. These two relative coordinates are viewed as two points in the \ReprName~network, and we can compute their signed distance field (SDF) values as: $d_1 = h(t_1,a_1,b_1, g(\Feat(t_1)) ), d_2 = h(t_2,a_2,b_2, g(\Feat(t_2)) )$ ($g,h$ are MLPs). The purpose of our method is to obtain a \textit{unique SDF value} for any point in the cylinder, so when $\AnotherPoint$ has two closest points, we simply define the SDF value of $\AnotherPoint$ is $d = \min (d_1, d_2)$. In fact, the point-wise minimum values of two SDFs are essentially representing the boolean union of the shapes of these two SDFs. For cases where a point has more than 2 closets points exist, its SDF value can be similarly defined. 

\subsection{Neural Generalized Cylinder}
% preprocessing: generate cylinders given curves. MLP structure, auto decoder training. positional encoding. Mesh extraction, quick filtering grid points. 

% \input{Supp/meso_skeleton}

\parahead{Preprocessing.}
% \re{For a given triangle mesh, the predicted skeleton curves can be very complicated if we use traditional skeleton-extraction algorithms. In Fig.~\ref{fig:supp_meso_skeleton}, we use meso-skeleton~\cite{meso_skeleton} with CGAL implementation for skeleton extraction, and it produces unsatisfying skeleton curves for users to control. In this case, only one center line is sufficient to represent the shape. Therefore, we mannually annotate skeleton curves for all 50 shapes, which can be seen in Fig.~\ref{fig:supp_fig_dataset}. } 

To fully cover the mesh with GCs with given skeleton curves, we first estimate the distance to the mesh for each point on the skeleton, denote as $r$ for point $\Point$. Then we directly set both $y$ and $z$ radii at $\Point$ to $k \cdot r$, where $k=1.1$ in our experiments. 

Next, to estimate the local frames of one curve, we first give a initial normalized vector $v_0$ at the endpoint $\Curve(0)$ of curve (e.g. set as the camera direction). Let $\mathbf{x}(0)$ be normalized tangent vector at $t=0$, then $\mathbf{y}(0),\mathbf{z}(0)$ in the local frame $\mathcal{F}(0)$ can be computed as:
\begin{align*}
    \hat{z}(0) &= v_0 - (v_0 \cdot \mathbf{x}(0)) \mathbf{x}(0), \\
    \mathbf{z}(0) &= \hat{z}(0) / \norm{\hat{z}(0)}_2, \\
    \mathbf{y}(0) &= \mathbf{z}(0) \times \mathbf{x}(0). \\
\end{align*}
Therefore, the local frames of a key frame can be computed from its previous key frame recursively. Assume $\mathbf{y}(t_i),\mathbf{z}(t_i)$ are computed at $t=t_i$, for $t=t_{i+1}$, $\mathbf{x}(t_{i+1})$ is selected as the normalized tangent vector at $t_{i+1}$, $\mathbf{y}(t_{i+1}), \mathbf{z}(t_{i+1})$ can be computed as:
\begin{align*}
    \hat{z}(t_{i+1}) &= \mathbf{z}(t_i) - (\mathbf{z}(t_i) \cdot \mathbf{x}(t_i)) \mathbf{x}(t_i), \\
    \mathbf{z}(t_{i+1}) &= \hat{z}(t_{i+1}) / \norm{\hat{z}(t_{i+1})}_2, \\
    \mathbf{y}(t_{i+1}) &= \mathbf{z}(t_{i+1}) \times \mathbf{x}(t_{i+1}). \\
\end{align*}
Thus GCs can be generated with \textit{interpolation} when radii and local frames of key frames are estimated for all curves. 

\parahead{Network architecture.}
We define one global feature vector $\GlobCode \in \mathbb{R}^{512}$ for one GC. The local feature $\Feat (t)$ for each point $\Curve(t) $on the central curve can be computed by $\Feat(t) = t\MLP_0(\GlobCode) + (1-t)\MLP_1(\GlobCode)$, and then we use $g(\Feat(t)$ for next SDF prediction network. Note that $\MLP_0, \MLP_1, g$ are multi-layer perceptrons (MLPs). Specifically, $\MLP_0, \MLP_1, g$ all have three layers with leaky ReLU as activation function and the latent dimension is also 512. To compute the neural SDF for a point $\Point$ with relative coordinates $(t,a,b)$, in practice, we actually first use positional encoding~\cite{mildenhall2020nerf} to embed $(t,a,b)$ into high dimensional space. Positional encoding is crucial in representing neural shape with high-frequency geometric details, and we use 6 frequencies for it (explanation in~\cite{mildenhall2020nerf}). Finally, we concatenate the feature $g(\Feat(t))$ and the embedded relative coordinates as the input to $h$, where $h$ is five-layer MLP with leaky ReLU activation and latent dimension of 512. The final layer of $h$ outputs the 1 dimensional SDF value, and it can be formulated as:

\begin{align*}
    F(\Point; z) = h(\textit{PosEnc}(t,a,b), g(\Feat(t)) ).
\end{align*}

\parahead{Mesh extraction.}
Since the neural SDF is only defined inside the GCs, we could utilize a quick pre-filtering of sampling points for faster mesh extraction with Marching Cubes. Specifically, a GC can be first approximated by a number of short straight cylinders (GCs with straight lines as their central curves). Then we can compute the bounding box of each straight cylinder, and filter out the sampling points inside this bounding box. This can be efficiently achieved for sampling points from a uniform 3D grid. In this way, all sampling points around the GC are filtered out and we compute the relative coordinates of these points to further determine they are inside the GC or not. In inference, the forward process of network is only done for points inside the GC, resulting in the acceleration of mesh extraction. 

\section{Experimental Details}
\label{supp_exp}
% formula of metrics(CD,HD,EMD); gallery of 50 shapes;
In this section, we will show implementation details of the networks and manipulation of \ReprName. 

\parahead{Metrics.}
To measure the error between the mesh extracted from neural SDF and the original mesh, we calculate their Chamfere Distance (CD), Hausdorff Distance (HD) and Earth Mover's Distance (EMD). Let $X$ be $N$ sample points and $Y$ be $M$ sample points, then CD and HD (we use an average version) between $X$ and $Y$ are formulated as:
\begin{align*}
    \textit{CD}(X,Y) &= \frac{1}{N} \sum_{\forall x \in X} \min_{\forall y \in Y} \norm{x - y}_2^2 + \frac{1}{M} \sum_{\forall y \in Y} \min_{\forall x \in X} \norm{x - y}_2^2, \\
    \textit{HD}(X,Y) &= \frac{1}{2} (\max_{\forall x \in X} \min_{\forall y \in Y} \norm{x - y}_2 + \max_{\forall y \in Y} \min_{\forall x \in X} \norm{x - y}_2).
\end{align*}
We refer the readers to~\cite{emd_pele2008} for formulation and implementation of EMD. In experiments, we uniformly sample $50,000$ points on the surface of two meshes, then calculate CD,HD and EMD. 

% \parahead{Representation Power.}
% \re{In Fig.~\ref{fig:supp_repr_power}, we show the case of armadillo reconstruction, where NGC with multiple GCs shows better performance on reconstruction of the hand than DeepSDF~\cite{deepsdf} and NGC with single NGC. Intuitively, multiple GCs (see Fig.~\ref{fig:supp_fig_dataset} for visualization of the skeleton) decompose the armadillo into several simple parts, which could be better approximated by the neural network.}  

% \input{Supp/repr_power}

\parahead{Dataset.}
Shapes in our experiments are from PSB dataset~\cite{PSB_dataset} and Objaverse~\cite{objaverse}. We show the reconstruction results and GC annotation in Fig.~\ref{fig:supp_fig_dataset}.

\parahead{Implementation details.}
In sampling, we sample inside the GCs, including surface samples and space samples. For surface samples, we first randomly sample around $50,000$ points on surface with Poisson Disk Sampling then add Gaussian noises($\mathcal{N}(0, \sigma^2)$) to these points along their normal direction as other $50,000$ surface samples, with noise level $\sigma = 0.01$. For all samples, the ground truth (GT) value of SDF to shape and relative coordinates are computed for training. 

For networks, the positional encoding module has 6 frequencies thus can map coordinates of $\mathbb{R}^3$ to embedding vectors of $\mathbb{R}^{39}$. In training, one batch consists of training data from 5 shapes, where $20,000$ space samples and $20,000$ surface samples are randomly picked from train set. After $10,000$ epochs of training (10 iterations for one epoch), the network can reconstruct shapes with high fidelity as shown in Fig.~\ref{fig:supp_fig_dataset}. For optimization, we use Adam optimizer with learning rate 1e-4 and train networks on one RTX3090 GPU. For mesh extraction from neural SDF, we use Marching Cubes to extract 0-level at resolution of $256^3$.

% manipulation: bezier curve, blend function definition, radius blending.
\parahead{Manipulation.}
As mentioned in the main paper, we control the shape by explicit GC manipulation. In experiments, we use Bezier curves and manipulate these curves by adjusting their control points. For radii and local frames, we simply change the value at key frames. 

Next, as stated, the shape blending can be done with the neural feature blending. Specifically, assume shape A has feature $\mathbf{u}(t)$ and shape B has feature $\mathbf{v}(t)$, then the blended feature $\textit{blend}(u,v,t)$ can be written as:
\begin{align*}
    \textit{blend}(\mathbf{u},\mathbf{v},t) = w(t) \mathbf{u}(t) + (1 - w(t)) \mathbf{v}(t), \quad  \forall t \in [0,1].
\end{align*}
Here $w(t)$ is a weight function, which can be specified by the users for their purpose. In our experiments, we use the truncated linear function, i.e., $w(t) = \min(\max(at+b, 0), 1)$. Parameters $a,b$ can be tuned for different effects of blending. When $a=1,b=0$, it degenerates to $w(t)=t$, which is simple linear blending of features. In practice, radius can also be blended for better visual effects, as shown in Fig.~\ref{fig:4_discussion_radius_blend}. This can be done by the same blending process, but feature $\mathbf{u}(t)$ is replaced with normalized radius, i.e. $\frac{(r_y(t), r_z(t)}{((r_y(t) + r_z(t)) / 2}$.

\begin{figure}
    \centering
    \includegraphics[width=0.7\linewidth]{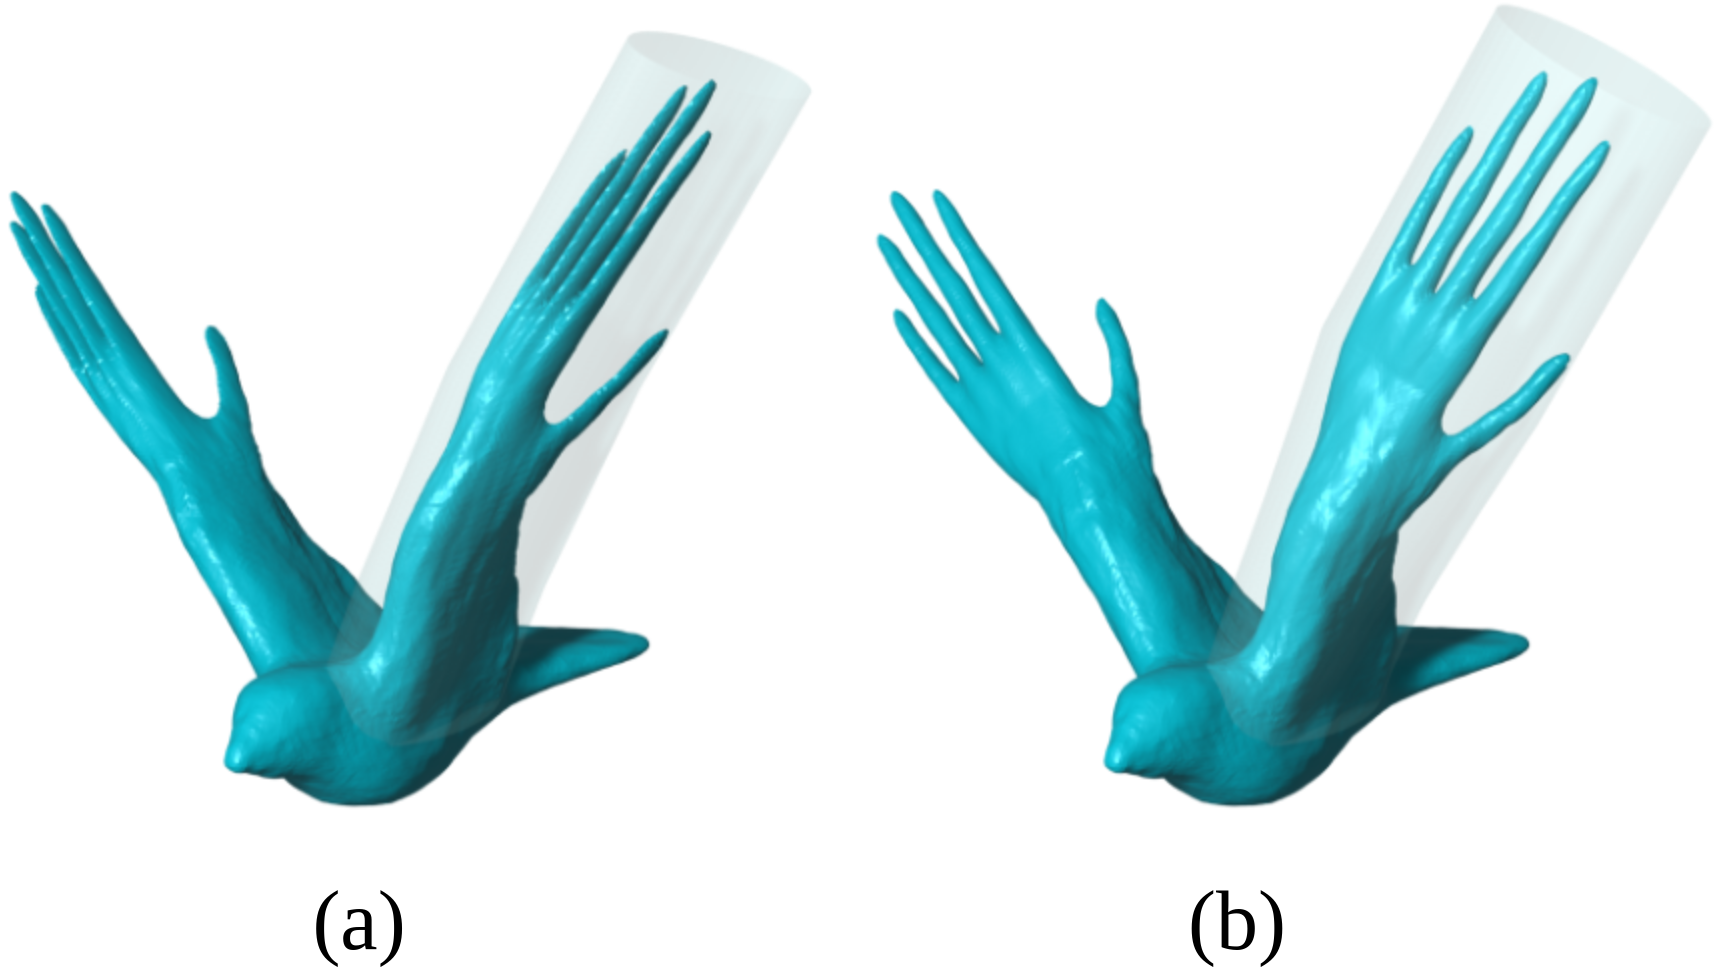}
    \caption{The effect of radius blending.}
    \label{fig:4_discussion_radius_blend}
\end{figure}

% generation framework...post processing..
\section{Shape Generation}
\label{supp_generation}
In this section, we introduce the details of shape generation with our \ReprName~representation in the experiment.

To adapt \ReprName~to generative models, we must first use one global feature vector to represent a shape, where the shape can have multiple GCs. We use RaBit~\cite{luo2023rabit} dataset for generation, which provides over 1500 shapes all in T-pose and with dense correspondence. Therefore, GCs of RaBit shapes have similar structures and can be automatically annotated. To represent the GCs of a shape, we pack the attributes at the key frame of the central curve as a vector, including curve point position, radius, and local frame. The vectors of all key frames thus can be learned by a MLP from a global feature vector. Similarly, the neural features (global latent vector $z$) of each central curve can be learned by another MLP from the global feature vector.

Next, we aim to construct a feature space, where any feature vector in this space is expected to represent a shape. Here we still adopt auto-decoder ~\cite{deepsdf} as the main learning framework. To further facilitate the learning of latent diffusion model, we follow~\cite{3DShape2VecSet} to use variational auto decoder (VAD). In VAD, the learnable global feature vector becomes a learnable feature distribution with a learnable mean vector and a learnable variance vector. Moreover, we use the KL-regularization in the loss function instead of the previous regularization. More details can be found in~\cite{3DShape2VecSet}.

Finally, we can train the latent diffusion model (LDM) on the feature space learned by VAD. We adopt the objective proposed in EDM~\cite{Karras2022edm}:
\begin{align*}
    \mathbb{E}_{\mathbf{n}_i \sim \mathcal{N}(\mathbf{0},\sigma^2 \mathbf{I})} \frac{1}{n} \sum_{i=1}^n
    \norm{\textit{Denoiser}(\Bar{z}_i + \mathbf{n}_i, \sigma) - \Bar{z}_i}_2^2.
\end{align*}

Here $\textit{Denoiser}$ is the denoising network in general diffusion models, and we use a six-layer transformer decoder for it in our experiments. $\Bar{z}_i$ is the sampling feature vector for $i^{th}$ shape. $\sigma$ is the noise level, and it is a random variable: $\ln(\sigma) \sim \mathcal{N}(P_{mean},P_{var})$. After training of LDM, we can generate feature vectors from Gaussian noises, by solving a stochastic differential equation with the high order Runge-Kutta method. These latent vectors then can be decoded as final shapes. More explanation and setting of parameters can be found in EDM~\cite{Karras2022edm}.
