# Supplementary material for: Controllable Shape Modeling with Neural Generalized Cylinder
Source: arXiv:2410.03675 source file (2024-09-18)
Supplement: Supplementary file 2 [file supp_fig_dataset.tex]

\begin{figure*}
    \centering
    \includegraphics[width=\linewidth]{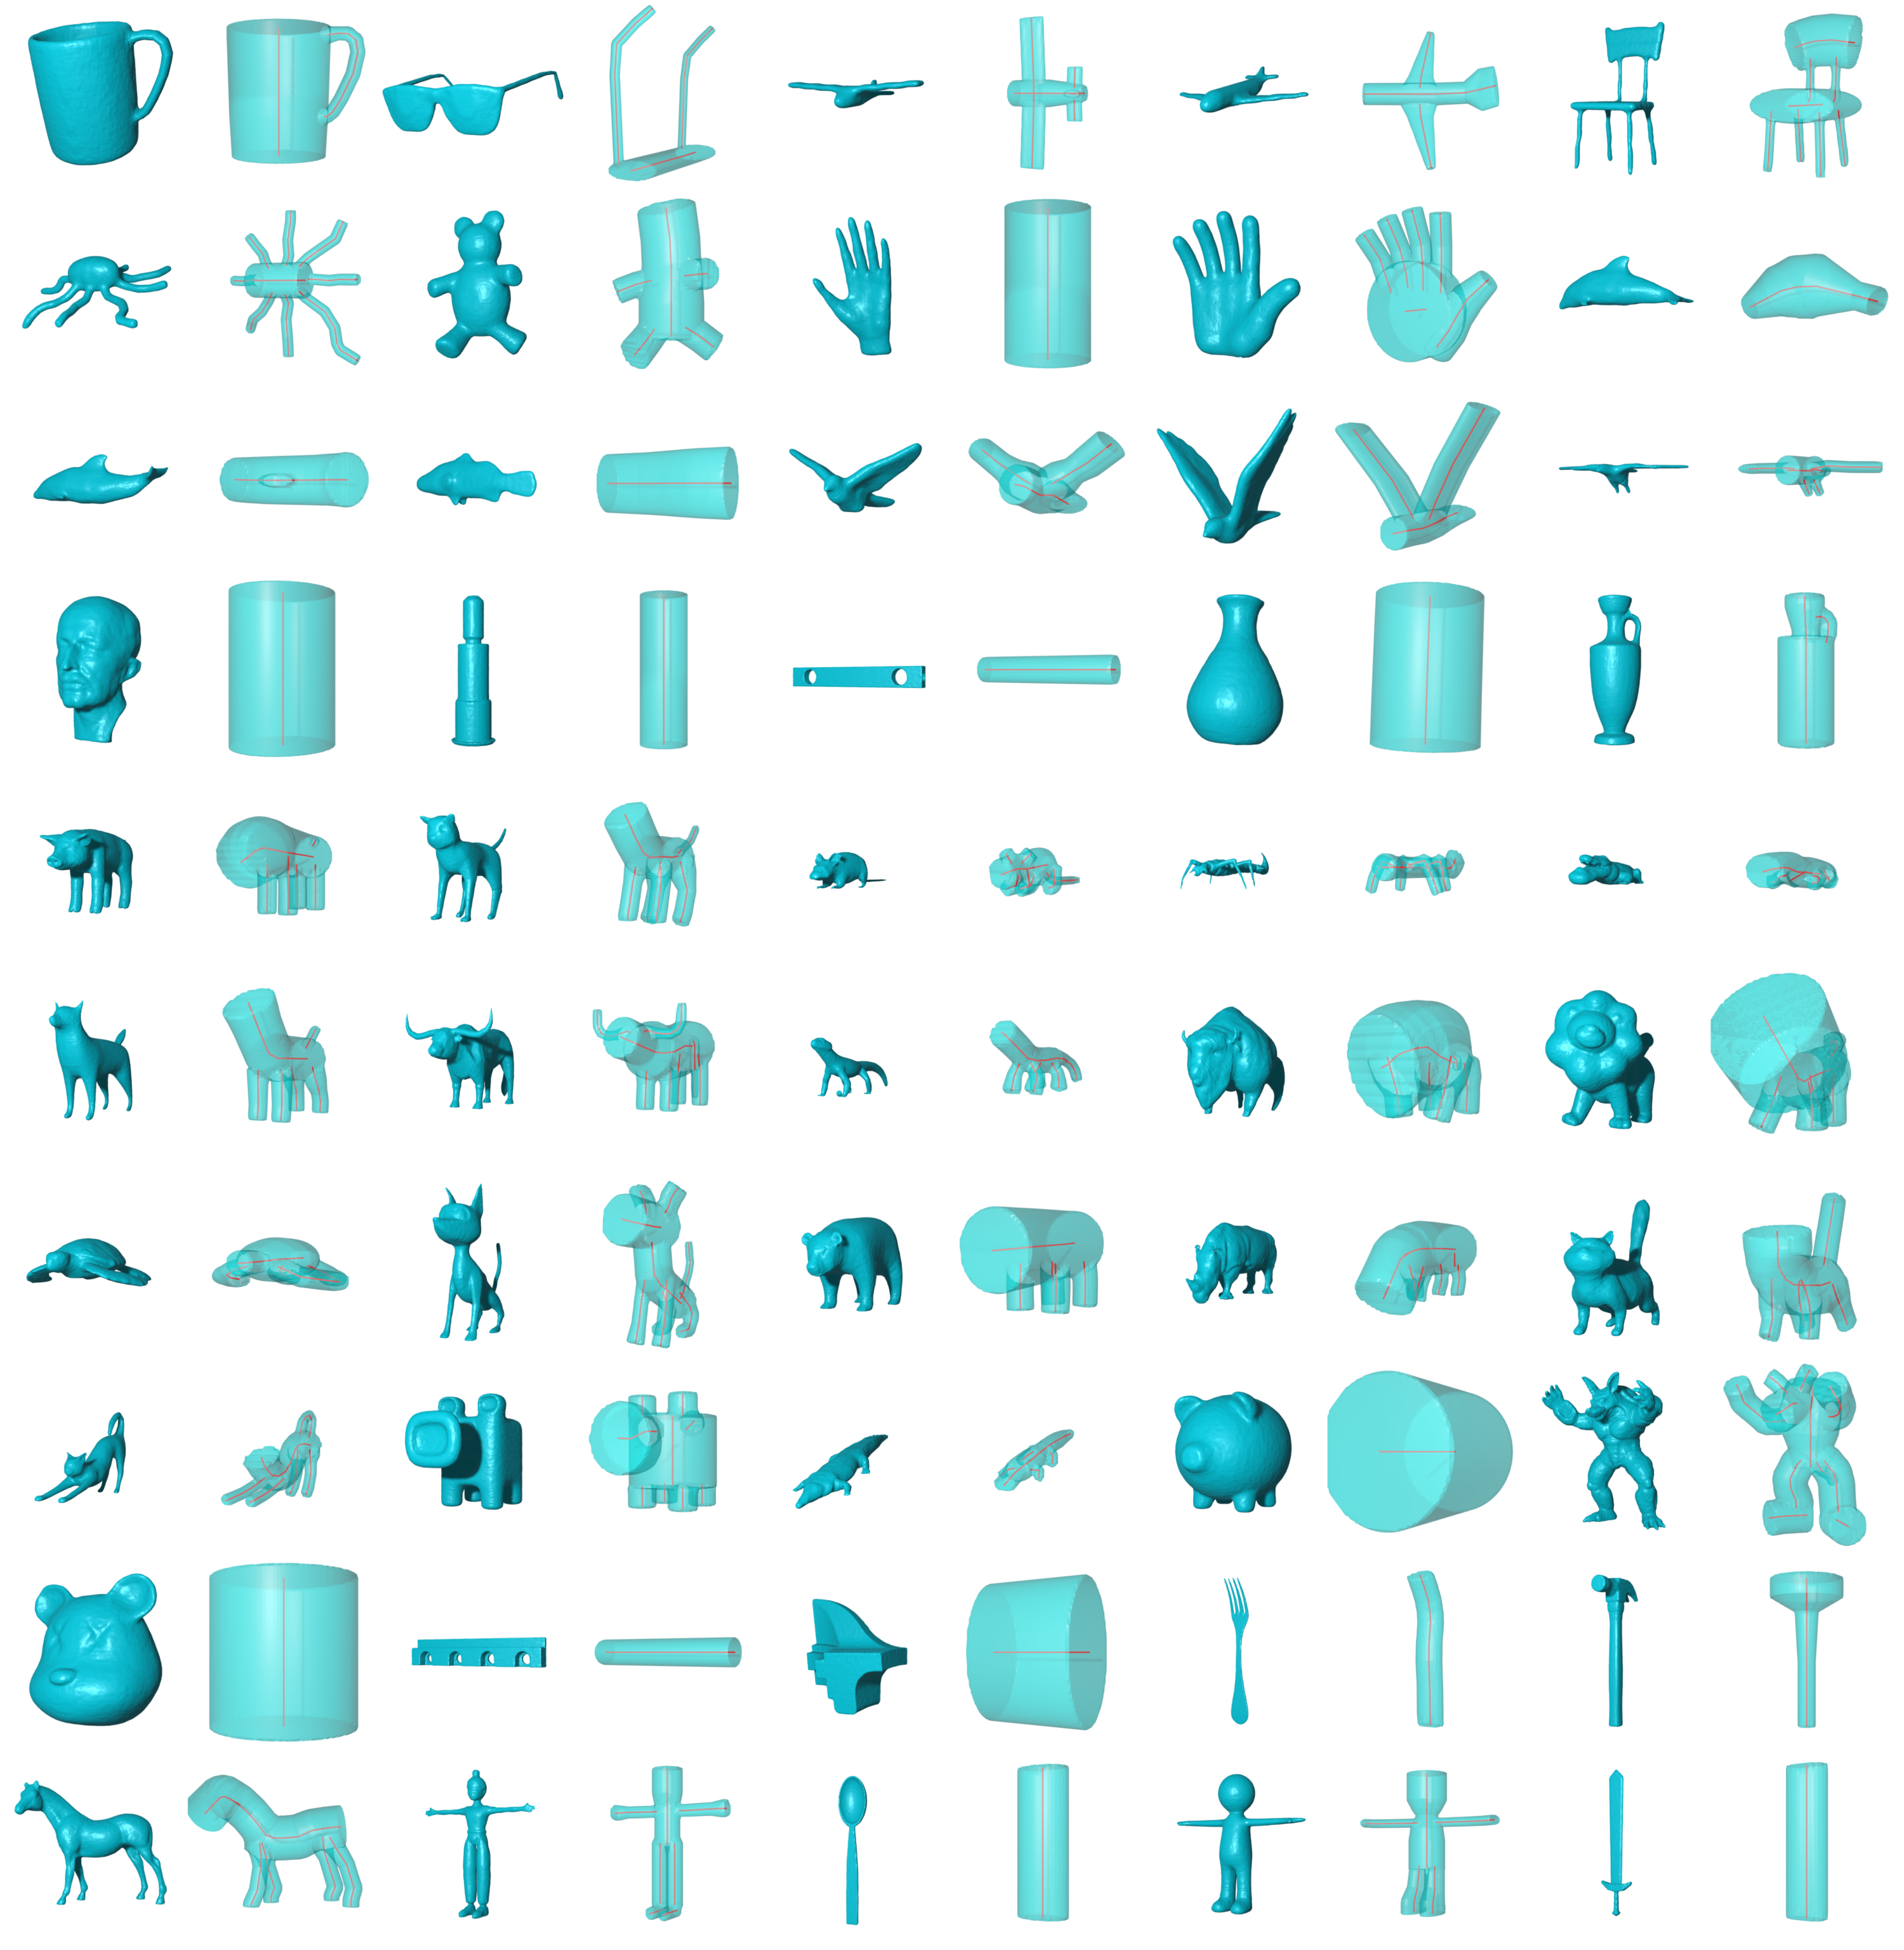}
    \caption{50 objects with their annotated generalized cylinders.}
    \label{fig:supp_fig_dataset}
\end{figure*}
